# Supplementary material for: Privacy-Enhanced Architecture for Occupancy-based HVAC Control
Source: arXiv:1607.03140 source file (2016-07-11)
Supplement: Supplementary file 1 [file appendix.tex]

We present a fast algorithm for evaluating adversarial location inference attacks. The idea is to formulate the exact MAP inference as an optimization problem over the variables
\begin{align}
\mathcal{Q} = \{&Q(X_k^{(m)})\in \mathbb{R}^{N+1},Q(X_{k-1}^{(m)},X_k^{(m)})\in\mathbb{R}^{(N+1)\times (N+1)},\nonumber\\
&Q(X_k^{(1)},\cdots,X_k^{(M)})\in \mathbb{R}^{N\times (M+1)}\}
\end{align}
These variables are indicators, so that
\begin{align}
&Q(X_k^{(m)})_n=1 \iff X_k^{(m)}=z_n\text{, for }n = 0,\cdots,N\\
&Q(X_{k-1}^{(m)},X_k^{(m)})_{n_1,n_2}=1 \iff X_{k-1}^{(m)}= z_{n_1},X_k^{(m)}=z_{n_2}\nonumber\\
&\text{for }n_1,n_2 = 0,\cdots,N\\ 
&Q(X_k^{(1)},\cdots,X_k^{(M)})_{n_3,i} = 1\iff \sum_{m=1}^M Q(X_k^{(m)})_{n_3}=i\nonumber\\
&\text{i.e., } Y_k^{n_3}= i\text{, for }n_3 = 1,\cdots,N\text{, }i = 0,\cdots,M
\end{align}

Some constraints $\mathcal{L}$ must be imposed on $\mathcal{Q}$ such that it has consistent meaning, which take the form 
\begin{align}
&\sum_n Q(X_k^{(m)})_n = 1\nonumber\\
&\sum_{n_1}Q(X_{k-1}^{(m)},X_k^{(m)})_{n_1,n_2}=Q(X_k^{(m)})_{n_2}\nonumber\\
&\sum_{n_2}Q(X_{k-1}^{(m)},X_k^{(m)})_{n_1,n_2}=Q(X_{k-1}^{(m)})_{n_1}\nonumber\\
& \sum_i Q(X_k^{(1)},\cdots,X_k^{(M)})_{n_3,i}= 1\nonumber\\
&\sum_iiQ(X_k^{(1)},\cdots,X_k^{(M)})_{n_3,i}=\sum_mQ(X_k^{(m)})_{n_3}
\end{align}
With these notations, MAP inference can now be cast as optimizing the log-likelihood of the FHMM model subject to the constraint that $\mathcal{Q}\in\mathcal{L}$ and that all the variables in $\mathcal{Q}$ take on binary values, which is represented by
\begin{align}
\min_{\mathcal{Q}\in \mathcal{L}\cap\{0,1\}} &-\sum_{n_3,k,i}\log \mathbb{P}(V_k^n|i)Q(X_k^{(1)},\cdots,X_k^{(M)})_{n_3,i}\nonumber\\
&-\sum_{m,k,n_1,n_2}Q(X_{k-1}^{(m)},X_k^{(m)})_{n_1,n_2}\log a_{n_1,n_2}
\end{align}
where $\mathbb{P}(V_k^n|i)$ is given by the occupancy distortion mechanism if the adversary knows the mechanism design; $\mathbb{P}(V_k^n|i)$ equals to identity matrix, otherwise. Now, we obtain an algorithm, as a substitute for Viterbi decoding, to perform adversarial location inference efficiently with many commercial MIP solvers.
